# Supplementary material for: A local limit theorem for random walks on the chambers of $\tilde{A}_2$ buildings
Source: arXiv:0912.1301 source file (2009-12-07)
Supplement: Supplementary file 1 [file supp-pdf.tex]

\endinput
